# Supplementary material for: New generation of effective core potentials from correlated calculations: 3d transition metal series
Source: arXiv:1805.06436 ancillary file (2018-05-16)
Supplement: Supplementary file 1 [file supplemental.pdf]

# Supplementary Material: A new generation of effective core potentials: 3d transition metal series

Abdulgani Annaberdiyev[1,*], Guangming Wang[1,*], Cody A. Melton[1,2,*], M. Chandler Bennett[1,2,*], Luke Shulenburger[2], and Lubos Mitas[1]

*1) Department of Physics,*

*North Carolina State University, Raleigh,*

*North Carolina 27695-8202, USA*

*and*

*2) Sandia National Laboratories,*

*Albuquerque, New Mexico 87123, USA*

*

(Dated: May 16, 2018)

PACS numbers:

## I. BASIS SETS

For each of the correlation consistent ECPs, (ccECP), we have constructed correlation consistent basis sets. To optimize the basis sets, we use the procedure of Balabanov *et al.*[1] to construct both cc-pV$n$Z and aug-cc-pV$n$Z basis sets for $n \in \{\mathrm{D}, \mathrm{T}, \mathrm{Q}, 5\}$ quality. We first optimize a set of primitive exponents for the $s, p, d$ functions using 13 primitives for the $s$ and $p$, and 11 primitives for the $d$. The optimal exponents are found by minimizing the HF energy for the [Ar]$3d^n4s^2$ state, which is the ground state for Sc-V, Mn-Ni, and Zn.

Once we have determined the optimal set of primitive exponents, we generate the minimal basis set by first minimizing the state-averaged HF energy for the [Ar]$3d^n4s^2$ state. This generates the first 2 $s$ contractions. For the first two $p$ contractions, we minimize the state-averaged HF energy of the [Ar]$3d^{n-1}4s^24p^1$ state. To generate the $d$ contraction, we consider a set of neutral states, namely the [Ar]$3d^n4s^2$, [Ar]$3d^{n+1}4s^1$, and [Ar]$3d^{n+2}$ states. We minimize the state-averaged HF energy of each of these states and obtain the contraction coefficients from the natural orbitals of the averaged density matrix from the individual state-averaged density matrices. This procedure provides two $s$, two $p$, and one $d$ contraction. To generate the cc-pV$n$Z basis, we must add an additional $n-1$ functions to the $s$, $p$, and $d$ levels as well as the polarization functions for the $f$, $g$, $h$, and $i$ functions (e.g. DZ has $1f$, TZ has $2f1g$, QZ has $3f2g1h$, and 5Z has $4f3g2h1i$). The additional $s$, $p$ and $d$ contracted functions are obtained from the averaged CISD density matrix from the [Ar]$3d^n4s^2$, [Ar]$3d^{n+1}4s^1$, and [Ar]$3d^{n+2}$ states. We ignore the first two natural orbitals for the $s$ and $p$ and first natural orbital for the $d$ from the averaged density matrix, and then take as the additional contracted functions the coefficients of the next highest occupation numbers (DZ takes the next highest, TZ takes the next two highest, QZ takes the next three highest, and 5Z takes the next four highest occupation number of the natural orbitals). The polarization functions are obtained from minimizing the average CISD energy of the [Ar]$3d^n4s^2$, [Ar]$3d^{n+1}4s^1$, and [Ar]$3d^{n+2}$ states. The polarization functions are even-tempered, i.e., we only optimize the smallest exponent and the ratio between the additional terms. Additionally, we also add an uncontracted function for the $s$, $p$, and $d$ basis sets using the smallest exponent that was in the original contraction, thus finalizing our cc-pV$n$Z basis sets.

Lastly, we generate the augmented basis set as follows. For the $s$, $p$, and $d$ functions, we take the smallest exponent and add an additional uncontracted function, with the exponent

being (roughly) a factor of two smaller than the smallest exponent. For the $f$, $g$, $h$, and $i$ functions, we use our optimized ratios from the even-tempered cc-pV$n$Z polarizations function to add an additional smaller exponent using the same ratio. For the terms that only have one exponent ($f$ for DZ, $g$ for TZ, $h$ for QZ, and $i$ for 5Z), we minimize the average CISD energy of the [Ar]$3d^n4s^2$, [Ar]$3d^{n+1}4s^1$, and [Ar]$3d^{n+2}$ states by adding an additional primitive exponent to be optimized. The final cc-pV$n$Z and aug-cc-pV$n$Z basis sets will be included on our website, `http://pseudopotentiallibrary.org`.

## II. ATOMIC SPECTRA

In the following subsections, we show the atomic excitation information and binding parameters for all molecule used in this work.

### A. Sc

Table II, shows atomic excitation discrepancies for Sc atom. ScH and ScO AE molecular parameters and corresponding discrepancies for various core approximations are shown in Table III and Table IV respectively.

TABLE I: Total energy components of the [Ar] $3d^14s^2$ $^2D$ ground state of the Sc atom using our ccECP.

| | T | Q | 5 | Extrap. | Numerical | Diffs |
|---|---|---|---|---|---|---|
| SCF | -46.119887 | -46.120165 | -46.120191 | -46.120194 | -46.120116 | -0.000078 |
| Correlation | -0.409235 | -0.422091 | -0.428269 | -0.435320 | | |

### B. Ti

In Table V, we give the total energy components for our ccECP of the Ti ground state. Table VI, shows atomic excitation discrepancies for Ti atom. TiH and TiO AE molecular parameters and corresponding discrepancies for various core approximations are shown in Table VII and Table VIII respectively.

TABLE II: Sc AE gaps and relative errors for various core approximations. All gaps are relative to the [Ar] $3d^1 4s^2$ $^2D$ state. All values in eV.

| Gaps | AE | UC | BFD | STU | eCEPP | ccECP.S |
|---|---|---|---|---|---|---|
| [Ar] $3d^2 4s^2$ $^3F$ | 0.509479 | 0.003048 | 0.525507 | 0.064818 | -0.000680 | 0.008299 |
| [Ar] $3d^2 4s^1$ $^4F$ | 1.419374 | 0.011864 | 0.671360 | 0.084764 | -0.002449 | 0.006857 |
| [Ar] $3d^3$ $^4F$ | 4.283618 | 0.011646 | 0.728095 | 0.152030 | -0.006531 | 0.008463 |
| [Ar] $3d^1 4s^1$ $^3D$ | 6.542273 | 0.002095 | 0.604447 | 0.028273 | -0.003293 | -0.009606 |
| [Ar] $3d^2$ $^3F$ | 7.144951 | 0.019375 | 0.705238 | 0.138533 | -0.000463 | -0.000408 |
| [Ar] $3d^1$ $^2D$ | 19.344148 | 0.004626 | 0.560909 | 0.105471 | 0.001551 | -0.021660 |
| [Ar] $^1S$ | 44.069078 | -0.040491 | 0.426239 | 0.123866 | -0.013715 | 0.002667 |
| [Ne] $3s^2$ $^1S$ | 795.976959 | -0.762055 | -0.281420 | 0.424253 | -2.238355 | 0.004354 |

TABLE III: ScH AE molecular binding parameters and discrepancies for various core approximations. All parameters were obtained using Morse potential fit. The parameters shown are dissociation energy $D_e$, equilibrium bond length $r_e$, vibrational frequency $\omega_e$ and dissociation energy discrepancy at dissociation bond length $D_{diss}$.

| | $D_e$(eV) | $r_e$(Å) | $\omega_e$(cm$^{-1}$) | $D_{diss}$(eV) |
|---|---|---|---|---|
| Exp. | 2.06[a] | 1.775[b] | 1547[b] | |
| AE | 2.30(1) | 1.755(5) | 1548(16) | |
| UC | 0.01(2) | 0.002(7) | -1(23) | 0.01(13) |
| BFD | 0.02(2) | 0.004(7) | 4(23) | 0.04(13) |
| STU | -0.01(2) | -0.003(7) | 3(23) | -0.00(13) |
| eCEPP | -0.00(2) | -0.001(7) | 1(23) | -0.00(13) |
| ccECP.S | -0.01(2) | -0.000(7) | -1(23) | 0.01(13) |

[a] Reference[2]

[b] Reference[3]

TABLE IV: ScO AE molecular binding parameters and discrepancies for various core approximations. Labeling as in Table III

| | $D_e$(eV) | $r_e$(Å) | $\omega_e$(cm$^{-1}$) | $D_{diss}$(eV) |
|---|---|---|---|---|
| Exp. | 7.07[a] | 1.668[a] | 965[a] | |
| AE | 6.95(1) | 1.659(1) | 975.6(7.1) | |
| UC | -0.01(2) | 0.002(2) | -2(10) | 0.06(22) |
| BFD | -0.08(2) | 0.008(2) | -4(10) | 0.42(24) |
| STU | -0.08(2) | -0.001(2) | -1(10) | 0.04(22) |
| eCEPP | 0.00(2) | 0.001(2) | -1(10) | 0.05(22) |
| ccECP.S | -0.01(2) | 0.000(2) | 0(10) | 0.04(22) |

[a] Reference[2]

TABLE V: Total energy components of the [Ar] $3d^2 4s^2$ $^3F$ ground state of the Ti atom using our ccECP.

| | T | Q | 5 | Extrap. | Numerical | Diffs |
|---|---|---|---|---|---|---|
| SCF | -57.606631 | -57.607057 | -57.607104 | -57.607110 | -57.607088 | -0.000022 |
| Correlation | -0.452225 | -0.467988 | -0.474562 | -0.482664 | | |

TABLE VI: Ti AE gaps and relative errors for various core approximations. All in eV.

| Gaps | | AE | UC | BFD | STU | eCEPP | ccECP |
|---|---|---|---|---|---|---|---|
| [Ar] $3d^3 4s^2$ | $^4F$ | 0.020661 | 0.008558 | 0.084231 | 0.073673 | 0.005225 | 0.007623 |
| [Ar] $3d^3 4s^1$ | $^5F$ | 0.796464 | 0.015718 | 0.110225 | 0.082066 | 0.006530 | 0.006560 |
| [Ar] $3d^4$ | $^5D$ | 3.616908 | 0.019344 | 0.185767 | 0.159201 | 0.009038 | 0.012720 |
| [Ar] $3d^2 4s^1$ | $^4F$ | 6.804955 | 0.003393 | 0.009862 | 0.026440 | -0.003403 | -0.009247 |
| [Ar] $3d^3$ | $^4F$ | 6.915550 | 0.026609 | 0.141649 | 0.141318 | 0.020958 | 0.006538 |
| [Ar] $3d^2$ | $^3F$ | 20.387116 | 0.009622 | 0.015878 | 0.112828 | 0.008137 | -0.017891 |
| [Ar] $3d^1$ | $^2D$ | 47.867620 | -0.037232 | -0.151758 | 0.130371 | -0.040542 | -0.029817 |
| [Ar] | $^1S$ | 91.091323 | -0.124071 | -0.391450 | 0.258178 | -1.234149 | 0.012368 |
| [Ne] $3s^2$ | $^1S$ | 1,028.587483 | -0.954480 | -0.171680 | 0.493782 | -1.703671 | 0.014604 |

TABLE VII: TiH AE molecular binding parameters and discrepancies for various core approximations. Labeling as in Table III

| | $D_e$(eV) | $r_e$(Å) | $\omega_e$(cm$^{-1}$) | $D_{diss}$(eV) |
|---|---|---|---|---|
| Exp. | 2.168$^a$ | 1.779$^a$ | 1405$^a$ | |
| AE | 2.105(4) | 1.762(2) | 1516.8(8.7) | |
| UC | -0.003(5) | 0.001(3) | -0(12) | 0.019(61) |
| BFD | -0.027(5) | 0.007(3) | -4(12) | 0.100(63) |
| STU | -0.045(5) | -0.000(3) | -3(13) | 0.046(61) |
| eCEPP | 0.005(5) | 0.000(3) | 2(12) | 0.006(60) |
| ccECP | 0.007(5) | 0.001(3) | 1(12) | 0.010(60) |

$^a$ Reference[2]

TABLE VIII: TiO AE molecular binding parameters and discrepancies for various core approximations. Labeling as in Table III

| | $D_e$(eV) | $r_e$(Å) | $\omega_e$(cm$^{-1}$) | $D_{diss}$(eV) |
|---|---|---|---|---|
| Exp. | 6.98$^a$ | 1.620$^a$ | 1009$^a$ | |
| AE | 6.85(1) | 1.615(2) | 999.1(6.8) | |
| UC | -0.01(2) | 0.002(3) | -2.0(9.6) | 0.06(22) |
| BFD | -0.10(2) | 0.007(3) | -4.1(9.9) | 0.41(24) |
| STU | -0.08(2) | -0.001(3) | -1.3(9.9) | 0.03(23) |
| eCEPP | 0.02(2) | 0.001(3) | 0.3(9.8) | 0.06(23) |
| ccECP | 0.00(2) | 0.000(3) | 1.0(9.7) | 0.02(22) |

$^a$ Reference[2]

### C. V

In Table IX, we give the total energy components for our ccECP of the V ground state. Table X, shows atomic excitation discrepancies for V atom. VH and VO AE molecular parameters and corresponding discrepancies for various core approximations are shown in Table XI and Table XII respectively.

TABLE IX: Total energy components of the [Ar] $3d^3 4s^2$ $^4F$ ground state of the V atom using our ccECP.

| | T | Q | 5 | Extrap. | Numerical | Diffs |
|---|---|---|---|---|---|---|
| SCF | -70.895598 | -70.896086 | -70.896115 | -70.896117 | -70.896038 | -0.000079 |
| Correlation | -0.503389 | -0.522224 | -0.529968 | -0.539407 | | |

TABLE X: V AE gaps and relative errors for various core approximations. All data in eV.

| Gaps | | AE | UC | BFD | STU | eCEPP | ccECP.S | ccECP |
|---|---|---|---|---|---|---|---|---|
| [Ar] $3d^4 4s^2$ | $^5D$ | -0.476250 | 0.010698 | 0.104690 | 0.069543 | -0.002350 | 0.005158 | 0.018813 |
| [Ar] $3d^4 4s^1$ | $^6D$ | 0.225411 | 0.016419 | 0.122574 | 0.072073 | -0.012547 | 0.000018 | 0.016268 |
| [Ar] $3d^5$ | $^6S$ | 2.477803 | 0.022536 | 0.223108 | 0.153314 | -0.012134 | 0.009320 | 0.040209 |
| [Ar] $3d^3 4s^1$ | $^5F$ | 7.040745 | 0.003875 | 0.011638 | 0.014400 | -0.012391 | -0.012788 | -0.005745 |
| [Ar] $3d^4$ | $^5D$ | 6.702435 | 0.028646 | 0.161530 | 0.123399 | 0.000007 | 0.003149 | 0.030633 |
| [Ar] $3d^3$ | $^4F$ | 21.353719 | 0.012672 | 0.037204 | 0.086384 | 0.004329 | -0.009391 | 0.011301 |
| [Ar] $3d^2$ | $^3F$ | 50.673774 | -0.030859 | -0.104118 | 0.088290 | -0.015417 | -0.022190 | -0.008337 |
| [Ar] $3d^1$ | $^2D$ | 97.385632 | -0.106347 | -0.297488 | 0.181266 | -0.065904 | -0.024749 | -0.014226 |
| [Ar] | $^1S$ | 162.607898 | -0.225926 | -0.639514 | 0.434473 | -1.746391 | 0.012854 | 0.026267 |
| [Ne] $3s^2$ | $^1S$ | 1,304.413862 | -1.135737 | 0.940843 | 1.273876 | -3.906868 | -0.005499 | 0.026110 |

### D. Cr

In Table XIII, we give the total energy components for our ccECP of the Cr ground state. Table XIV, shows atomic excitation discrepancies for Cr atom. CrH and CrO AE molecular parameters and corresponding discrepancies for various core approximations are shown in Table XV and Table XVI respectively.

### E. Mn

In Table XVII, we give the total energy components for our ccECP of the Mn ground state. Table XVIII, shows atomic excitation discrepancies for Mn atom. MnH and MnO

TABLE XI: VH AE molecular binding parameters and discrepancies for various core approximations. Labeling as in Table III

| | $D_e$(eV) | $r_e$(Å) | $\omega_e$(cm$^{-1}$) | $D_{diss}$(eV) |
|---|---|---|---|---|
| Exp. | 2.229$^a$ | | | |
| | 2.229(69)$^b$ | 1.730$^b$ | | |
| | 2.28(19),2.433(65)$^c$ | 1.73$^c$ | | |
| AE | 2.622(2) | 1.6799(9) | 1652.7(3.7) | |
| UC | 0.011(3) | -0.001(1) | 2.9(5.2) | -0.016(29) |
| BFD | -0.035(3) | 0.005(1) | -3.7(5.4) | 0.101(31) |
| STU | -0.035(3) | -0.000(1) | -2.7(5.4) | 0.034(30) |
| eCEPP | 0.016(3) | 0.000(1) | 2.3(5.1) | -0.011(28) |
| ccECP.S | 0.033(3) | -0.002(1) | 5.3(5.2) | -0.045(29) |
| ccECP | 0.009(3) | -0.000(1) | 2.1(5.2) | -0.008(29) |

$^a$ Reference[2]

$^b$ Reference[4]

$^c$ Reference[5]

AE molecular parameters and corresponding discrepancies for various core approximations are shown in Table XIX and Table XX respectively.

### F. Fe

In Table XXI, we give the total energy components for our ccECP of the Fe ground state. Table XXII, shows atomic excitation discrepancies for Fe atom. FeH and FeO AE molecular parameters and corresponding discrepancies for various core approximations are shown in Table XXIII and Table XXIV respectively.

### G. Co

In TableXXV, we give the total energy components for our ccECP of the Co ground state. Table XXVI, shows atomic excitation discrepancies for Co atom. CoH and CoO AE

TABLE XII: VO AE molecular binding parameters and discrepancies for various core approximations. Labeling as in Table III

| | $D_e$(eV) | $r_e$(Å) | $\omega_e$(cm$^{-1}$) | $D_{diss}$(eV) |
|---|---|---|---|---|
| Exp. | 6.505$^a$ | 1.589$^a$ | 1011$^a$ | |
| | 6.548(87)$^b$ | 1.589$^b$ | | |
| | 6.548(87),6.474$^c$ | 1.589$^c$ | | |
| AE | 6.686(9) | 1.585(2) | 1005.1(5.1) | |
| UC | -0.00(1) | 0.002(2) | -1.4(7.2) | 0.05(18) |
| BFD | -0.10(1) | 0.005(3) | -3.1(7.5) | 0.32(19) |
| STU | -0.06(1) | -0.003(2) | 2.2(7.3) | -0.04(18) |
| eCEPP | 0.01(1) | 0.002(2) | -1.0(7.3) | 0.08(18) |
| ccECP.S | 0.03(1) | -0.001(2) | 2.9(7.3) | -0.04(18) |
| ccECP | 0.02(1) | -0.001(2) | 3.2(7.3) | -0.03(18) |

$^a$ Reference[2]

$^b$ Reference[4]

$^c$ Reference[5]

TABLE XIII: Total energy components of the [Ar] $3d^5 4s^1$ $^7S$ ground state of the Cr atom for our ccECP.

| | T | Q | 5 | Extrap. | Numerical | Diffs |
|---|---|---|---|---|---|---|
| SCF | -86.047811 | -86.048454 | -86.048542 | -86.048556 | -86.048401 | -0.000155 |
| Correlation | -0.542224 | -0.566030 | -0.575994 | -0.586753 | | |

molecular parameters and corresponding discrepancies for various core approximations are shown in Table XXVII and Table XXVIII respectively.

### H. Ni

In Table XXIX, we show the total energy components for the Ni ground state using our ccECP. Table XXX, shows atomic excitation discrepancies for Ni atom. NiH and NiO AE

TABLE XIV: Cr AE gaps and relative errors for various ECPs. All values in eV

| Gaps | | AE | UC | BFD | STU | eCEPP | ccECP.S | ccECP |
|---|---|---|---|---|---|---|---|---|
| [Ar] $3d^5 4s^2$ | $^6S$ | -1.639160 | 0.008708 | 0.100464 | 0.075539 | 0.002912 | 0.002231 | -0.007320 |
| [Ar] $3d^5 4s^1$ | $^7S$ | -1.026768 | 0.012626 | 0.109308 | 0.070858 | -0.002395 | -0.001850 | -0.015864 |
| [Ar] $3d^6$ | $^5D$ | 3.444963 | 0.006449 | 0.189582 | 0.145908 | -0.006204 | -0.002068 | -0.024681 |
| [Ar] $3d^4 4s^1$ | $^6D$ | 7.256491 | 0.003483 | 0.003102 | 0.016517 | -0.016762 | -0.011701 | -0.017497 |
| [Ar] $3d^5$ | $^6S$ | 5.735591 | 0.023783 | 0.139894 | 0.140656 | 0.010259 | 0.016681 | -0.005632 |
| [Ar] $3d^4$ | $^5D$ | 22.265020 | 0.013198 | 0.032490 | 0.127077 | -0.010531 | 0.006177 | -0.003946 |
| [Ar] $3d^3$ | $^4F$ | 53.342070 | -0.022558 | -0.082097 | 0.181337 | -0.015293 | -0.003129 | 0.008626 |
| [Ar] $3d^2$ | $^3F$ | 102.464577 | -0.084655 | -0.217174 | 0.344850 | 0.022232 | -0.012436 | 0.032518 |
| [Ar] $3d^1$ | $^2D$ | 171.920939 | -0.176820 | -0.446866 | 0.669754 | 0.143731 | -0.017361 | 0.082695 |
| [Ar] | $^1S$ | 262.444038 | -0.312659 | -1.402775 | 1.242200 | 0.422348 | 0.020817 | 0.217202 |
| [Ne] $3s^2$ | $^1S$ | 1,627.174829 | -1.275153 | 2.973117 | 0.528908 | 0.506350 | 0.036490 | -2.483884 |

molecular parameters and corresponding discrepancies for various core approximations are shown in Table XXXI and Table XXXII respectively.

### I. Cu

In Table XXXIII, we show the total energy components for the Cu atom ground state using our ccECP. Table XXXIV, shows atomic excitation discrepancies for Cu atom. CuH and CuO AE molecular parameters and corresponding discrepancies for various core approximations are shown in Table XXXV and Table XXXVI respectively.

### J. Zn

In Table XXXVII, we show the total energy components for the Zn atom ground state using our ccECP. Table XXXVIII, shows atomic excitation discrepancies for Zn atom. ZnH and ZnO AE molecular parameters and corresponding discrepancies for various core approximations are shown in Table XXXIX and Table XL respectively.

TABLE XV: CrH AE molecular binding parameters and discrepancies for various core approximations. Labeling as in Table III

| | $D_e$(eV) | $r_e$(Å) | $\omega_e$(cm$^{-1}$) | $D_{diss}$(eV) |
|---|---|---|---|---|
| Exp. | 2.029[a] | 1.656[a] | 1581[a] | |
| | 2.029(69)[b] | 1.656[b] | | |
| | 2.11(14),2.238(65)[c] | 1.656[c] | | |
| AE | 2.120(6) | 1.614(2) | 1740(13) | |
| UC | 0.015(8) | 0.003(3) | -8(17) | -0.004(73 |
| BFD | 0.057(7) | 0.005(3) | -7(16) | -0.038(70) |
| STU | 0.024(7) | 0.002(3) | -9(16) | -0.037(69) |
| eCEPP | 0.019(7) | 0.005(3) | -14(16) | -0.002(70) |
| ccECP.S | 0.028(7) | 0.004(3) | -12(16) | -0.018(69) |
| ccECP | 0.013(7) | 0.005(3) | -13(16) | -0.002(70) |

[a] Reference[2]

[b] Reference[4]

[c] Reference[5]

TABLE XVI: CrO AE molecular binding parameters and discrepancies for various core approximations. Labeling as in Table III

| | $D_e$(eV) | $r_e$(Å) | $\omega_e$(cm$^{-1}$) | $D_{diss}$(eV) |
|---|---|---|---|---|
| Exp. | 4.467[a] | 1.615[a] | 898[a] | |
| | 4.540(52)[b] | 1.621[b] | | |
| | 4.818(87)[c] | 1.615[c] | | |
| AE | 4.573(4) | 1.6139(6) | 899.2(1.9) | |
| UC | 0.008(5) | 0.0010(9) | -0.2(2.9) | 0.024(52) |
| BFD | 0.090(5) | -0.0044(9) | 9.8(2.9) | -0.146(51) |
| STU | -0.012(6) | -0.0024(9) | 2.0(3.0) | -0.043(54) |
| eCEPP | 0.018(5) | 0.0011(9) | 0.2(2.9) | 0.018(52) |
| ccECP.S | 0.041(5) | -0.0025(9) | 4.8(2.9) | -0.079(51) |
| ccECP | 0.010(5) | -0.0009(9) | 1.5(2.9) | -0.027(51) |

[a] Reference[2]

[b] Reference[4]

[c] Reference[5]

TABLE XVII: Total energy components of the [Ar] $3d^5 4s^2$ $^6S$ ground state of the Mn atom for our ccECP.

| | T | Q | 5 | Extrap. | Numerical | Diffs |
|---|---|---|---|---|---|---|
| SCF | -103.243494 | -103.244240 | -103.244299 | -103.244305 | -103.244161 | -0.000144 |
| Correlation | -0.591277 | -0.617442 | -0.628553 | -0.642432 | | |

TABLE XVIII: Mn AE gaps and relative error for various core approximations. All in eV.

| Gaps | | AE | UC | BFD | STU | eCEPP | ccECP.S | ccECP |
|---|---|---|---|---|---|---|---|---|
| [Ar] $3d^6 4s^2$ | $^5D$ | 1.299360 | 0.001050 | 0.146607 | 0.028564 | 0.004187 | -0.003555 | -0.006144 |
| [Ar] $3d^6 4s^1$ | $^6D$ | 2.151429 | 0.006575 | 0.169347 | 0.010605 | 0.002082 | -0.006991 | -0.013559 |
| [Ar] $3d^7$ | $^4F$ | 5.772304 | 0.007078 | 0.285947 | 0.059634 | 0.018798 | 0.004177 | -0.003478 |
| [Ar] $3d^5 4s^1$ | $^7S$ | 7.414670 | 0.003239 | -0.003639 | -0.004177 | -0.006771 | -0.008937 | -0.008985 |
| [Ar] $3d^6$ | $^5D$ | 9.245516 | 0.007056 | 0.194099 | 0.017318 | 0.003874 | -0.015398 | -0.013276 |
| [Ar] $3d^5$ | $^6S$ | 23.059159 | 0.014572 | 0.022398 | 0.081569 | 0.014290 | 0.030141 | 0.050613 |
| [Ar] $3d^4$ | $^5D$ | 56.822155 | -0.015390 | -0.072555 | 0.256077 | -0.026524 | 0.016815 | 0.033293 |
| [Ar] $3d^3$ | $^4F$ | 108.315370 | -0.074830 | -0.158482 | 0.600224 | -0.059576 | 0.010784 | 0.017702 |
| [Ar] $3d^2$ | $^3F$ | 180.815120 | -0.162619 | -0.291000 | 1.159615 | -0.070647 | 0.003077 | 0.004779 |
| [Ar] $3d^1$ | $^2D$ | 276.392004 | -0.282966 | -0.586852 | 1.989336 | -0.043384 | -0.008268 | 0.013606 |
| [Ar] | $^1S$ | 395.519402 | -0.451819 | -1.184772 | 3.166735 | 0.029970 | 0.001807 | 0.103825 |
| [Ne] $3s^2$ | $^1S$ | 2001.865958 | -1.490682 | 3.394075 | 0.790442 | -2.370058 | 0.004111 | -6.624472 |

TABLE XIX: MnH AE molecular binding parameters and discrepancies for various core approximations. Labeling as in Table III

| | $D_e$(eV) | $r_e$(Å) | $\omega_e$(cm$^{-1}$) | $D_{diss}$(eV) |
|---|---|---|---|---|
| Exp. | 1.349[a] | 1.731[a] | 1548[a] | |
| AE | 1.644(5) | 1.721(3) | 1521(18) | |
| UC | -0.002(7) | 0.000(5) | -0(26) | 0.004(90) |
| BFD | 0.067(7) | -0.008(4) | 27(26) | -0.100(87) |
| STU | -0.035(7) | 0.002(5) | -13(26) | 0.034(91) |
| eCEPP | 0.016(7) | -0.001(4) | 5(26) | -0.021(89) |
| ccECP.S | 0.027(7) | -0.004(4) | 10(26) | -0.048(88) |
| ccECP | 0.002(7) | -0.001(5) | 0(26) | -0.009(90) |

[a] Reference[2]

TABLE XX: MnO AE molecular binding parameters and discrepancies for various core approximations. Labeling as in Table III

| | $D_e$(eV) | $r_e$(Å) | $\omega_e$(cm$^{-1}$) | |
|---|---|---|---|---|
| Exp. | 3.881[a] | 1.646[a] | 840[a] | |
| AE | 3.773(9) | 1.640(2) | 841.1(4.8) | |
| UC | -0.01(1) | 0.001(2) | -0.2(6.6) | 0.03(11) |
| BFD | -0.01(1) | -0.003(2) | 1.0(6.1) | -0.06(10) |
| STU | -0.09(1) | 0.001(2) | -8.2(6.7) | 0.05(11) |
| eCEPP | 0.02(1) | -0.000(2) | 2.6(6.6) | -0.01(11) |
| ccECP.S | 0.04(1) | -0.004(2) | 6.8(6.6) | -0.11(11) |
| ccECP | 0.01(1) | -0.002(2) | 3.3(6.7) | -0.03(11) |

[a] Reference[2]

TABLE XXI: Total energy components of the [Ar] $3d^6 4s^2$ $^5D$ ground state of the Fe atom.

| | T | Q | 5 | Extrap. | Num. | Diffs |
|---|---|---|---|---|---|---|
| SCF | -122.641201 | -122.642105 | -122.642174 | -122.642183 | -122.641993 | -0.000190 |
| Correlation | -0.677200 | -0.708431 | -0.719770 | -0.732173 | | |

TABLE XXII: Fe AE gaps and relative errors for various ECPs. All data in eV

| Gaps | | AE | UC | BFD | STU | eCEPP | ccECP.S | ccECP |
|---|---|---|---|---|---|---|---|---|
| [Ar]$4s^2 3d^7$ | $^4F$ | -0.057987 | 0.001660 | 0.156504 | 0.044160 | 0.011820 | 0.007696 | -0.005231 |
| [Ar] $4s^1 3d^7$ | $^5F$ | 0.888551 | 0.006370 | 0.171349 | 0.033548 | 0.008323 | -0.002355 | -0.014157 |
| [Ar] $3d^8$ | $^3F$ | 4.157110 | 0.010139 | 0.291230 | 0.092898 | 0.030171 | -0.003989 | -0.017050 |
| [Ar] $4s^1 3d^6$ | $^6D$ | 7.885826 | 0.004183 | 0.001180 | 0.005114 | -0.004736 | -0.020115 | -0.015930 |
| [Ar] $3d^7$ | $^4F$ | 8.162522 | 0.016486 | 0.199663 | 0.071353 | 0.026536 | 0.002202 | -0.002154 |
| [Ar]$3d^6$ | $^5D$ | 24.090858 | 0.014936 | 0.033942 | 0.099740 | 0.010690 | 0.008389 | 0.013777 |
| [Ar]$3d^5$ | $^6S$ | 54.661521 | -0.005615 | -0.168899 | 0.206248 | -0.017071 | 0.004946 | 0.021878 |
| [Ar]$3d^4$ | $^5D$ | 109.577638 | -0.051901 | -0.192542 | 0.455601 | -0.007441 | -0.005419 | -0.008571 |
| [Ar]$3d^3$ | $^4F$ | 185.022592 | -0.129771 | -0.222149 | 0.890969 | 0.067005 | -0.000924 | -0.005565 |
| [Ar]$3d^2$ | $^3F$ | 284.232562 | -0.235873 | -0.354853 | 1.557802 | 0.247372 | 0.001835 | 0.040188 |
| [Ar]$3d^1$ | $^2D$ | 409.151353 | -0.374283 | -0.745345 | 2.506921 | 0.518200 | -0.005224 | 0.160413 |
| [Ar] | $^1S$ | 560.024014 | -0.563164 | -1.561520 | 3.821096 | 0.924669 | 0.002865 | 0.431303 |
| [Ne]$3s^2$ | $^1S$ | 2,426.492957 | -1.657243 | 3.573802 | 0.956335 | -0.680726 | -0.017867 | -5.966712 |

TABLE XXIII: FeH AE molecular binding parameters and discrepancies for various core approximations. Labeling as in Table III

| | $D_e$(eV) | $r_e$(Å) | $\omega_e$(cm$^{-1}$) | $D_{diss}$(eV) |
|---|---|---|---|---|
| Exp. | 1.70[a] | 1.589[a] | 1827[a] | |
| | 1.600(35)[b] | 1.630[c] | | |
| | 1.712(13),1.943(65)[d] | 1.63[d] | | |
| AE | 1.89(1) | 1.538(4) | 1833(28) | |
| UC | -0.01(2) | -0.003(7) | 14(42) | 0.01(15) |
| BFD | -0.09(2) | -0.006(7) | 17(44) | 0.09(16) |
| STU | -0.05(2) | -0.006(7) | 11(43) | 0.02(15) |
| eCEPP | -0.00(2) | -0.002(6) | 9(41) | 0.00(15) |
| ccECP.S | 0.00(2) | -0.004(6) | 13(41) | -0.01(14) |
| ccECP | -0.00(2) | -0.002(6) | 9(41) | -0.00(14) |

[a] Reference[2]

[b] Reference[4]

[c] Reference[5]

TABLE XXIV: FeO AE molecular binding parameters and discrepancies for various core approximations. Labeling as in Table III

| | $D_e$(eV) | $r_e$(Å) | $\omega_e$(cm$^{-1}$) | $D_{diss}$(eV) |
|---|---|---|---|---|
| Exp. | 4.224[a] | 1.616[a] | 880[a] | |
| AE | 4.12(1) | 1.611(3) | 878.7(8.2) | |
| UC | -0.01(2) | 0.001(4) | -1(11) | 0.03(19) |
| BFD | -0.04(2) | -0.003(4) | 1(11) | -0.04(19) |
| STU | -0.07(2) | -0.003(4) | -0(12) | -0.02(20) |
| eCEPP | 0.02(2) | 0.000(4) | 2(12) | -0.00(20) |
| ccECP.S | 0.06(2) | -0.004(4) | 6(11) | -0.13(19) |
| ccECP | 0.03(2) | -0.001(4) | 3(12) | -0.03(19) |

[a] Reference[2]

TABLE XXV: Total energy components of the [Ar] $3d^7 4s^2$ $^4F$ ground state of the Co atom using our ccECP.

| | T | Q | 5 | Extrap. | Numerical | Diffs |
|---|---|---|---|---|---|---|
| SCF | -144.325544 | -144.327075 | -144.327246 | -144.327268 | -144.327074 | -0.000194 |
| Correlation | -0.746000 | -0.782672 | -0.799273 | -0.820951 | | |

TABLE XXVI: Co AE gaps and relative errors in eV

| Gaps | | AE | UC | BFD | STU | ccECP.S | ccECP |
|---|---|---|---|---|---|---|---|
| [Ar] $3d^8 4s^2$ | $^3F$ | -0.648824 | 0.003846 | 0.138580 | 0.038570 | 0.003500 | -0.011140 |
| [Ar] $3d^8 4s^1$ | $^4F$ | 0.404998 | 0.008382 | 0.146827 | 0.029158 | 0.000131 | -0.018138 |
| [Ar] $3d^9$ | $^2D$ | 3.290224 | 0.013495 | 0.245172 | 0.082758 | 0.001712 | -0.027850 |
| [Ar] $3d^7 4s^1$ | $^5F$ | 8.285103 | 0.004751 | -0.004194 | 0.008731 | -0.007956 | -0.014990 |
| [Ar] $3d^8$ | $^3F$ | 7.852169 | 0.016852 | 0.154921 | 0.060521 | 0.007556 | -0.012459 |
| [Ar] $3d^7$ | $^4F$ | 24.959596 | 0.014340 | 0.012356 | 0.096283 | 0.010968 | 0.005804 |
| [Ar] $3d^6$ | $^5D$ | 58.474931 | -0.000315 | -0.137538 | 0.215407 | 0.000966 | 0.010511 |
| [Ar] $3d^5$ | $^6S$ | 109.967312 | -0.035818 | -0.288764 | 0.449440 | -0.020260 | 0.016728 |
| [Ar] $3d^4$ | $^5D$ | 189.676472 | -0.096964 | -0.229092 | 0.878645 | -0.018478 | 0.002135 |
| [Ar] $3d^3$ | $^4F$ | 292.523396 | -0.190846 | -0.217323 | 1.539629 | 0.001712 | 0.062171 |
| [Ar] $3d^2$ | $^3F$ | 421.774512 | -0.312948 | -0.383028 | 2.475055 | 0.017756 | 0.218327 |
| [Ar] $3d^1$ | $^2D$ | 579.286933 | -0.467425 | -0.905317 | 3.738709 | 0.010326 | 0.520393 |
| [Ar] | $^1S$ | 765.100530 | -0.673798 | -1.957082 | 5.417765 | -0.013019 | 1.067807 |
| [Ne] $3s^2$ | $^1S$ | 2910.339236 | -1.819632 | 5.795586 | 1.122129 | -0.018151 | -8.537068 |

TABLE XXVII: CoH AE molecular binding parameters and discrepancies for various core approximations. Labeling as in Table III

| | $D_e$(eV) | $r_e$(Å) | $\omega_e$(cm$^{-1}$) | $D_{diss}$(eV) |
|---|---|---|---|---|
| Exp. | 2.099$^a$ | 1.52$^a$ | 1925$^a$ | |
| | 1.973(52)$^b$ | 1.530$^b$ | | |
| | 2.19(13),2.368(65)$^c$ | 1.53$^c$ | | |
| AE | 2.123(4) | 1.515(2) | 1813(12) | |
| UC | -0.006(5) | -0.000(3) | 1(17) | 0.008(67) |
| BFD | -0.133(6) | -0.002(3) | 1(21) | 0.155(80) |
| STU | -0.042(6) | -0.003(3) | 2(18) | 0.029(69) |
| ccECP.S | 0.010(5) | -0.002(2) | 7(17) | -0.021(66) |
| ccECP | 0.014(5) | 0.000(2) | 2(17) | -0.008(65) |

[a] Reference[2]

[b] Reference[4]

[c] Reference[5]

TABLE XXVIII: CoO AE molecular binding parameters and discrepancies for various core approximations. Labeling as in Table III

| | $D_e$(eV) | $r_e$(Å) | $\omega_e$(cm$^{-1}$) | $D_{diss}$(eV) |
|---|---|---|---|---|
| Exp. | 3.998$a$ | 1.616$^a$ | 880$^a$ | |
| AE | 3.79(2) | 1.607(5) | 891(16) | |
| UC | 0.00(3) | 0.001(7) | -2(22) | 0.02(35) |
| BFD | 0.01(3) | -0.009(7) | 13(23) | -0.16(35) |
| STU | -0.06(3) | -0.005(7) | 3(23) | -0.05(35) |
| ccECP.S | 0.05(3) | -0.004(7) | 8(23) | -0.12(35) |
| ccECP | 0.01(3) | -0.000(7) | 1(22) | 0.00(35) |

[a] Reference[2]

TABLE XXIX: Total energy components for the [Ar]$3d^8 4s^2$ $^3F$ state of the Ni atom for our ccECP.

| SCF | T | Q | 5 | Extrap. | Numerical | Diffs |
|---|---|---|---|---|---|---|
| SCF | -168.409192 | -168.411003 | -168.411106 | -168.411112 | -168.410808 | -0.000304 |
| Correlation | -0.822084 | -0.864373 | -0.883557 | -0.908639 | | |

TABLE XXX: Ni AE gaps and relative errors for various ECPs. All values in eV

| Gaps | | AE | UC | BFD | STU | ccECP.S | ccECP |
|---|---|---|---|---|---|---|---|
| [Ar] $3d^9 4s^2$ | $^2D$ | -1.209029 | 0.005065 | 0.146336 | 0.013536 | -0.003339 | 0.000304 |
| [Ar] $3d^9 4s^1$ | $^3D$ | -0.039999 | 0.010094 | 0.154368 | -0.007817 | -0.003776 | -0.003715 |
| [Ar] $3d^{10}$ | $^1S$ | 1.665329 | 0.014848 | 0.258005 | 0.022213 | -0.004163 | -0.006370 |
| [Ar] $3d^8 4s^1$ | $^4F$ | 8.678287 | 0.004880 | -0.004271 | -0.026728 | 0.001234 | -0.011767 |
| [Ar] $3d^9$ | $^2D$ | 7.580538 | 0.017010 | 0.152086 | -0.041737 | 0.002174 | -0.002632 |
| [Ar] $3d^8$ | $^3F$ | 25.813278 | 0.013459 | -0.005649 | -0.039091 | 0.014570 | -0.007257 |
| [Ar] $3d^7$ | $^4F$ | 61.040014 | -0.000243 | -0.144218 | 0.100049 | 0.016374 | -0.042470 |
| [Ar] $3d^6$ | $^5D$ | 116.199196 | -0.026699 | -0.226084 | 0.435981 | 0.004456 | -0.105248 |
| [Ar] $3d^5$ | $^6S$ | 192.239024 | -0.075327 | -0.281178 | 1.016989 | -0.018535 | -0.175304 |
| [Ar] $3d^4$ | $^5D$ | 300.110087 | -0.148578 | -0.080333 | 2.014774 | -0.012141 | -0.209976 |
| [Ar] $3d^3$ | $^4F$ | 433.615540 | -0.256215 | 0.003373 | 3.416095 | 0.010293 | -0.172026 |
| [Ar] $3d^2$ | $^3F$ | 596.091441 | -0.391620 | -0.212840 | 5.276018 | 0.023892 | -0.054807 |
| [Ar] $3d^1$ | $^2D$ | 789.334381 | -0.559135 | -0.961215 | 7.649629 | 0.010737 | 0.163535 |
| [Ar] | $^1S$ | 1013.195350 | -0.779566 | -2.452519 | 10.611841 | -0.013917 | 0.540565 |
| [Ne] $3s^2$ | $^1S$ | 3455.730422 | -1.969547 | 5.538940 | 20.075182 | -0.001036 | -13.848153 |

TABLE XXXI: NiH AE molecular binding parameters and discrepancies for various core approximations. Labeling as in Table III

| | $D_e$(eV) | $r_e$(Å) | $\omega_e$(cm$^{-1}$) | $D_{diss}$(eV) |
|---|---|---|---|---|
| Exp. | 2.6582$^a$ | 1.475$^a$ | 1927$^a$ | |
| AE | 3.249(2) | 1.4502(7) | 2039.3(5.7) | |
| UC | -0.014(3) | -0.0004(9) | 2.6(7.7) | 0.024(39) |
| BFD | -0.122(2) | -0.0045(8) | 11.3(6.7) | 0.130(34) |
| STU | -0.025(3) | 0.001(1) | -10.9(8.1) | -0.001(40) |
| ccECP.S | 0.004(3) | -0.002(1) | 6.9(7.9) | -0.022(40) |
| ccECP | 0.031(3) | -0.001(1) | 2.9(8.2) | -0.056(41) |

$^a$ Reference[2]

TABLE XXXII: NiO AE molecular binding parameters and discrepancies for various core approximations. Labeling as in Table III

| | $D_e$(eV) | $r_e$(Å) | $\omega_e$(cm$^{-1}$) | $D_{diss}$(eV) |
|---|---|---|---|---|
| Exp. | 3.92$^a$ | 1.627$^a$ | 838$^a$ | |
| AE | 4.23(1) | 1.619(2) | 863.7(7.3) | |
| UC | -0.00(1) | 0.002(3) | -3(10) | 0.02(18) |
| BFD | -0.04(2) | -0.012(4) | 20(14) | -0.08(23) |
| STU | -0.01(2) | -0.004(4) | 4(12) | -0.09(20) |
| ccECP.S | 0.06(2) | -0.004(4) | 6(11) | -0.14(18) |
| ccECP | 0.02(2) | 0.000(4) | 2(11) | 0.01(19) |

$^a$ Reference[2]

TABLE XXXIII: Total energy components of the [Ar] $3d^{10}4s^1$ $^2S$ ground state of the Cu atom using our ccECP.

| | T | Q | 5 | Extrap. | Numerical | Diffs |
|---|---|---|---|---|---|---|
| SCF | -195.335042 | -195.337118 | -195.337366 | -195.337400 | -195.336990 | -0.000410 |
| Correlation | -0.957822 | -1.008029 | -1.030905 | -1.060903 | | |

TABLE XXXIV: Cu AE and relative errors for various core approximations. All values in eV

| Gaps | AE | UC | BFD | STU | eCEPP | ccECP.S | ccECP |
|---|---|---|---|---|---|---|---|
| [Ar] $3d^{10}4s^2$ $^1S$ | -2.760729 | 0.004101 | 0.053157 | 0.039397 | -0.000870 | -0.016530 | -0.006277 |
| [Ar] $3d^{10}4s^1$ $^2S$ | -1.513939 | 0.007503 | 0.047758 | 0.042300 | 0.004682 | -0.020428 | -0.007892 |
| [Ar] $3d^9 4s^1$ $^3D$ | 9.062324 | 0.005137 | -0.006833 | 0.004934 | 0.003888 | -0.003649 | -0.002273 |
| [Ar] $3d^{10}$ $^1S$ | 6.223451 | 0.013241 | 0.014972 | 0.047085 | 0.003103 | -0.032589 | -0.008363 |
| [Ar] $3d^9$ $^2D$ | 26.646257 | 0.012720 | -0.009051 | 0.024636 | 0.003493 | -0.009803 | 0.010994 |
| [Ar] $3d^8$ $^3F$ | 63.558190 | -0.000543 | -0.027268 | 0.020881 | 0.003248 | 0.010925 | 0.017731 |
| [Ar] $3d^7$ $^4F$ | 121.008477 | -0.025039 | -0.028883 | 0.055165 | 0.013036 | 0.018442 | -0.001066 |
| [Ar] $3d^6$ $^5D$ | 201.489726 | -0.062319 | -0.024452 | 0.156973 | 0.047778 | 0.010412 | -0.036229 |
| [Ar] $3d^5$ $^6S$ | 305.535974 | -0.122740 | -0.058675 | 0.364107 | 0.118660 | -0.008278 | -0.054449 |
| [Ar] $3d^4$ $^5D$ | 444.867210 | -0.207748 | 0.024219 | 0.733521 | 0.331561 | -0.002246 | -0.067000 |
| [Ar] $3d^3$ $^4F$ | 612.257887 | -0.328280 | -0.034713 | 1.317769 | 0.665239 | 0.022817 | 0.031193 |
| [Ar] $3d^2$ $^3F$ | 811.134546 | -0.476918 | -0.377656 | 2.138293 | 1.124162 | 0.032874 | 0.255770 |
| [Ar] $3d^1$ $^2D$ | 1043.247944 | -0.657795 | -1.166121 | 3.235735 | 1.709602 | 0.012528 | 0.655110 |
| [Ar] $^1S$ | 1308.271906 | -0.893022 | -2.520960 | 4.697743 | 2.455655 | -0.013314 | 1.337623 |
| [Ne] $3s^2$ $^1S$ | 4066.688500 | -2.130124 | 8.869749 | 5.120704 | 15.171119 | -0.025267 | -13.809237 |

TABLE XXXV: CuH AE molecular binding parameters and discrepancies for various core approximations. Labeling as in Table III

| | $D_e$(eV) | $r_e$(Å) | $\omega_e$(cm$^{-1}$) | $D_{diss}$(eV) |
|---|---|---|---|---|
| Exp. | 2.749[a] | 1.463[a] | 1941[a] | |
| | 2.715(61)[b] | 1.463[a] | | |
| | 2.736(208)[c] | 1.463[a] | | |
| AE | 2.83(3) | 1.47(1) | 1937(52) | |
| UC | -0.00(4) | -0.00(2) | 1(73) | 0.00(40) |
| BFD | 0.02(4) | -0.00(2) | 4(74) | -0.05(40) |
| STU | 0.01(4) | -0.00(2) | 6(73) | -0.03(40) |
| eCEPP | 0.02(4) | -0.00(2) | 8(73) | -0.04(40) |
| ccECP.S | 0.00(4) | -0.00(2) | 2(73) | -0.02(40) |
| ccECP | -0.01(4) | 0.00(2) | 1(73) | 0.02(40) |

[a] Reference[2]

[b] Reference[4]

[c] Reference[5]

TABLE XXXVI: CuO AE molecular binding parameters and discrepancies for various core approximations. Labeling as in Table III

| | $D_e$(eV) | $r_e$(Å) | $\omega_e$(cm$^{-1}$) | $D_{diss}$(eV) |
|---|---|---|---|---|
| Exp. | 2.888[a] | 1.724[a] | 640[a] | |
| AE | 2.769(7) | 1.731(3) | 651.5(5.8) | |
| UC | -0.01(1) | 0.001(4) | -0.3(8.3) | 0.01(13) |
| BFD | 0.04(1) | -0.008(4) | 1.6(8.6) | -0.20(12) |
| STU | -0.01(1) | -0.006(4) | 4.1(9.1) | -0.07(13) |
| eCEPP | 0.05(1) | -0.007(4) | 6.0(8.6) | -0.14(13) |
| ccECP.S | 0.01(1) | -0.003(4) | -0.4(8.5) | -0.07(13) |
| ccECP | -0.02(1) | 0.001(4) | -2.1(8.4) | 0.02(13) |

[a] Reference[2]

TABLE XXXVII: Total energy components for the [Ar] $3d^{10}4s^2$ $^1S$ ground state of the Zn atom using our ccECP.

| | T | Q | 5 | Extrap. | Numerical | Diffs |
|---|---|---|---|---|---|---|
| SCF | -225.274095 | -225.274983 | -225.275051 | -225.275057 | -225.274600 | -0.000457 |
| Correlation | -0.977277 | -1.030767 | -1.055331 | -1.087707 | | |

TABLE XXXVIII: Zn AE gaps and relative errors for various ECPs. All values in eV

| Gaps | | AE | UC | BFD | STU | ccECP.S | ccECP |
|---|---|---|---|---|---|---|---|
| [Ar] $3d^{10}4s^1$ | $^2S$ | 9.411709 | 0.004952 | 0.018765 | 0.004463 | 0.007538 | 0.000215 |
| [Ar] $3d^9 4s^2$ | $^2D$ | 17.323005 | -0.009362 | -0.205955 | -0.022585 | 0.009686 | 0.022019 |
| [Ar] $3d^{10}$ | $^1S$ | 27.392261 | 0.011411 | 0.036333 | 0.006989 | 0.002052 | -0.009078 |
| [Ar] $3d^9$ | $^2D$ | 67.262367 | 0.003722 | -0.050548 | 0.003788 | 0.010425 | 0.013184 |
| [Ar] $3d^8$ | $^3F$ | 126.975193 | -0.018903 | -0.090639 | 0.051139 | 0.013474 | 0.028731 |
| [Ar] $3d^7$ | $^4F$ | 210.344966 | -0.052708 | -0.055643 | 0.173830 | 0.006980 | 0.031967 |
| [Ar] $3d^6$ | $^5D$ | 319.614848 | -0.099359 | 0.033786 | 0.406930 | -0.008892 | 0.026004 |
| [Ar] $3d^5$ | $^6S$ | 455.004148 | -0.170049 | 0.098292 | 0.795761 | -0.026917 | 0.025026 |
| [Ar] $3d^4$ | $^5D$ | 629.026722 | -0.264676 | 0.351989 | 1.415417 | -0.015099 | 0.072364 |
| [Ar] $3d^3$ | $^4F$ | 833.485035 | -0.396401 | 0.369407 | 2.316968 | 0.018092 | 0.171157 |
| [Ar] $3d^2$ | $^3F$ | 1,071.906266 | -0.556213 | -0.076598 | 3.529685 | 0.034067 | 0.296417 |
| [Ar] $3d^1$ | $^2D$ | 1,346.006047 | -0.748315 | -2.414393 | 5.101447 | 0.007904 | 0.438073 |
| [Ar] | $^1S$ | 1,655.288042 | -0.996097 | -3.118490 | 7.132298 | -0.032440 | 0.638571 |
| [Ne] $3s^2$ | $^1S$ | 4,748.163279 | -2.271911 | 7.708246 | 5.787312 | -0.022816 | -8.705975 |

TABLE XXXIX: ZnH AE molecular binding parameters and discrepancies for various core approximations. Labeling as in Table III

| | $D_e$(eV) | $r_e$(Å) | $\omega_e$(cm$^{-1}$) | $D_{diss}$(eV) |
|---|---|---|---|---|
| Exp. | 0.951[a] | 1.595[a] | 1608[a] | |
| | 0.937(22)[b] | 1.590[b] | | |
| | 0.945(22)[c] 1.595[a] | | | |
| AE | 0.928(5) | 1.580(3) | 1614(35) | |
| UC | -0.002(7) | 0.000(4) | -1(49) | 0.002(86) |
| BFD | 0.060(7) | -0.014(4) | 56(50) | -0.113(81) |
| STU | 0.006(7) | -0.002(4) | 6(49) | -0.016(85) |
| ccECP.S | 0.031(7) | -0.006(4) | 27(49) | -0.053(84) |
| ccECP | 0.012(7) | -0.002(4) | 9(49) | -0.020(85) |

[a] Reference[6]

[b] Reference[4]

[c] Reference[5]

TABLE XL: ZnO AE molecular binding parameters and discrepancies for various core approximations. Labeling as in Table III

| | $D_e$(eV) | $r_e$(Å) | $\omega_e$(cm$^{-1}$) | $D_{diss}$(eV) |
|---|---|---|---|---|
| Exp. | | | 720[a] | |
| | 1.644(39)[b] | 1.800[b] | | |
| | 1.657(43)[c] | 1.8[b] | | |
| AE | 1.46(2) | 1.697(9) | 669(22) | |
| UC | -0.01(3) | 0.00(1) | -2(31) | 0.02(27) |
| BFD | 0.05(3) | -0.01(1) | 16(31) | -0.16(25) |
| STU | -0.02(3) | -0.00(1) | -0(31) | -0.03(26) |
| ccECP.S | 0.02(3) | -0.00(1) | 6(31) | -0.06(26) |
| ccECP | 0.00(3) | -0.00(1) | 0(31) | -0.01(26) |

[a] Reference[7]

[b] Reference[4]

[c] Reference[5]

* These authors contributed equally to this work

[1] N. B. Balabanov and K. A. Peterson, The Journal of Chemical Physics **123**, 064107 (2005), https://doi.org/10.1063/1.1998907, URL `https://doi.org/10.1063/1.1998907`.

[2] F. Furche and J. P. Perdew, The Journal of chemical physics **124**, 044103 (2006).

[3] R. Ram and P. Bernath, The Journal of chemical physics **105**, 2668 (1996).

[4] X. Xu, W. Zhang, M. Tang, and D. G. Truhlar, Journal of chemical theory and computation **11**, 2036 (2015).

[5] Z. Fang, M. Vasiliu, K. A. Peterson, and D. A. Dixon, Journal of chemical theory and computation **13**, 1057 (2017).

[6] K. Huber and G. Herzbery, *Molecular spectra and molecular structure: IV. Constants of diatomic molecules* (Van Nostrand Reinhold Co., 1979).

[7] V. D. Moravec, S. A. Klopcic, B. Chatterjee, and C. C. Jarrold, Chemical physics letters **341**, 313 (2001).
